# Supplementary material for: Enabling Versatile Controls for Video Diffusion Models
Source: arXiv:2503.16983 source file (2025-03-21)
Supplement: Supplementary file 1 [file x_suppl.tex]

\clearpage
\setcounter{page}{1}
\maketitlesupplementary

\section{Additional Results}

\subsection{Qualitative Comparison} 
\begin{figure}
    \vspace{-3pt}
    \centering
    \includegraphics[width=1\linewidth]{./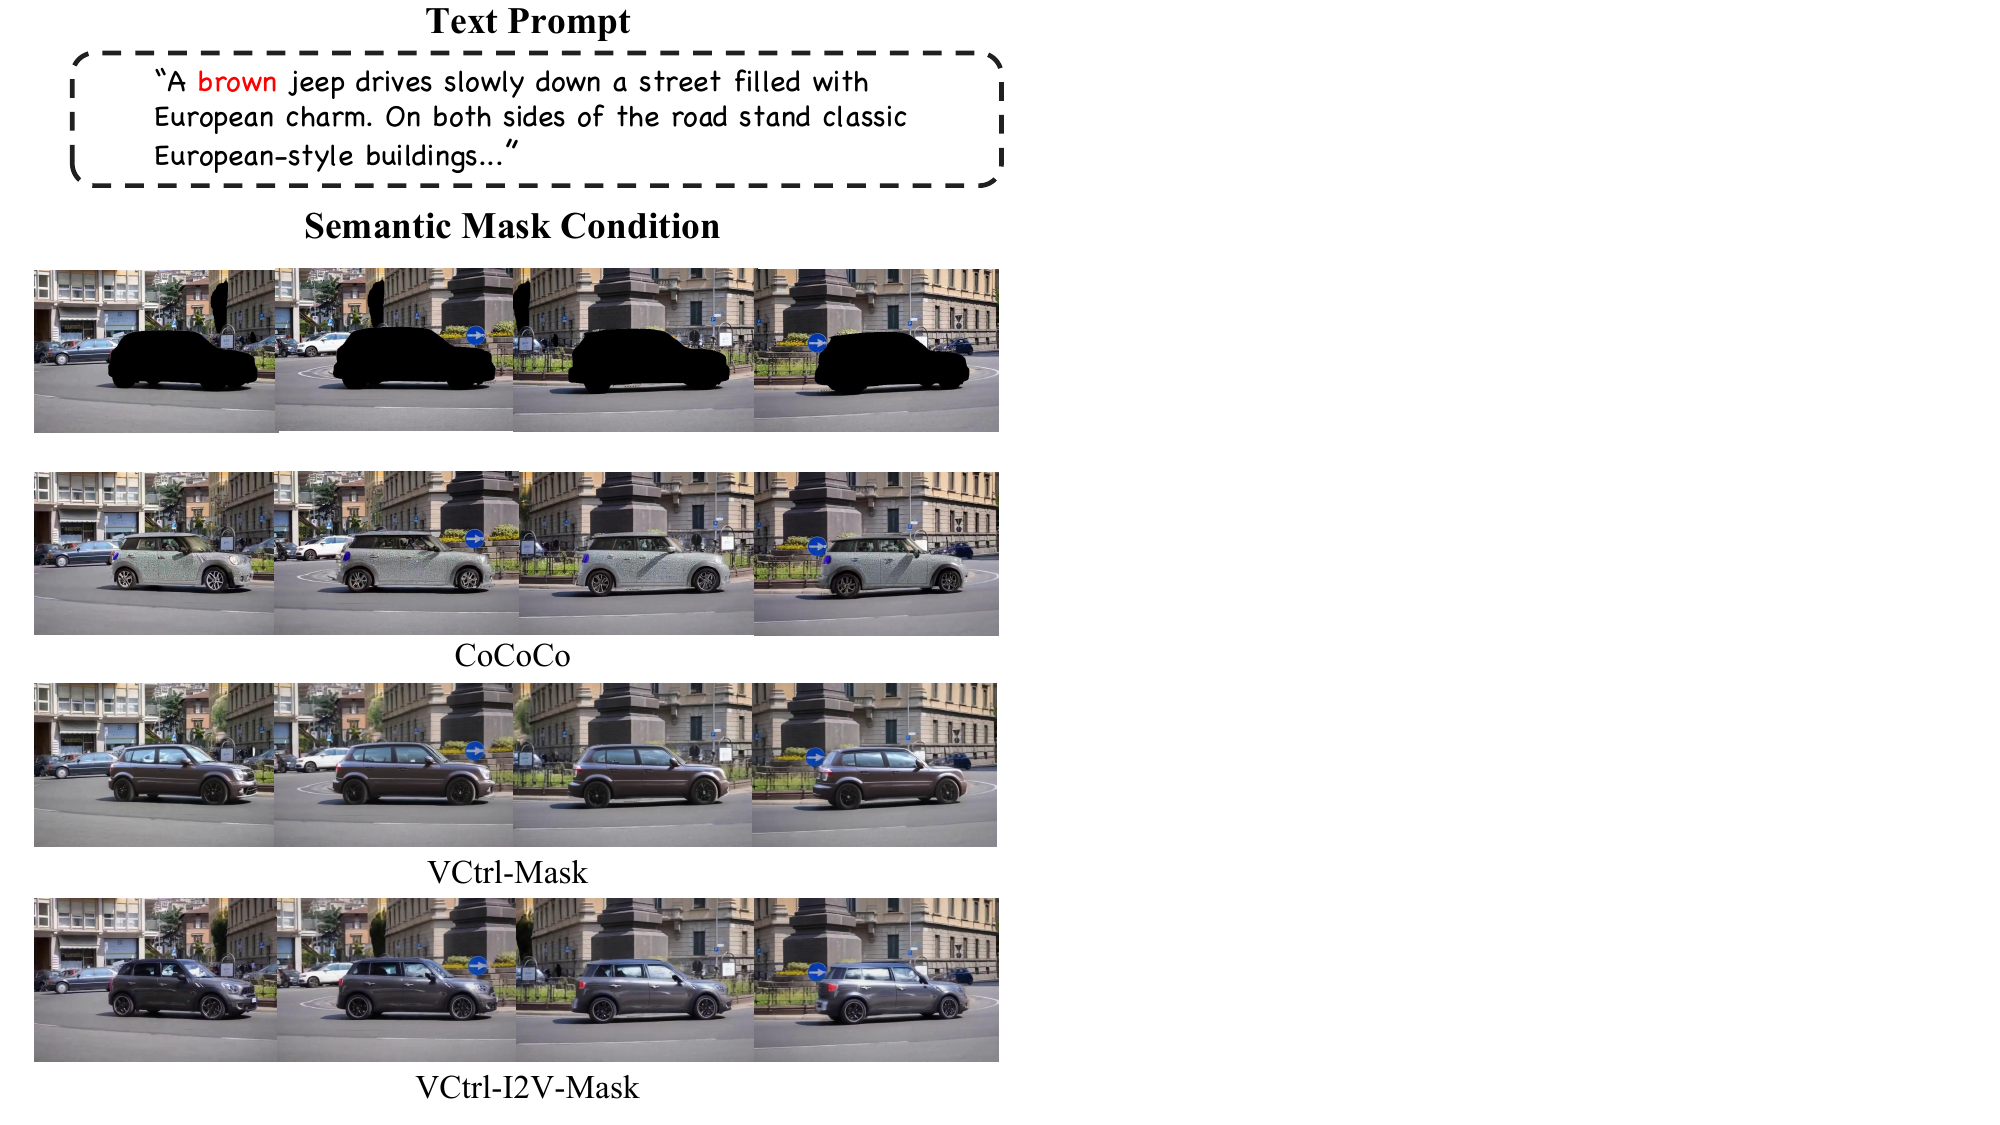}
    \vspace{-20pt}
    \caption{\textbf{Qualitative comparison to previous methods.} We compare our method with CoCoCo~\cite{zi2024cococo}, demonstrating superior object consistency and stronger temporal coherence to the segmentation mask conditions.}
    \vspace{-7pt}
    \label{fig:mask_task}
\end{figure}
\begin{figure}
    \vspace{-3pt}
    \centering
    \includegraphics[width=1\linewidth]{./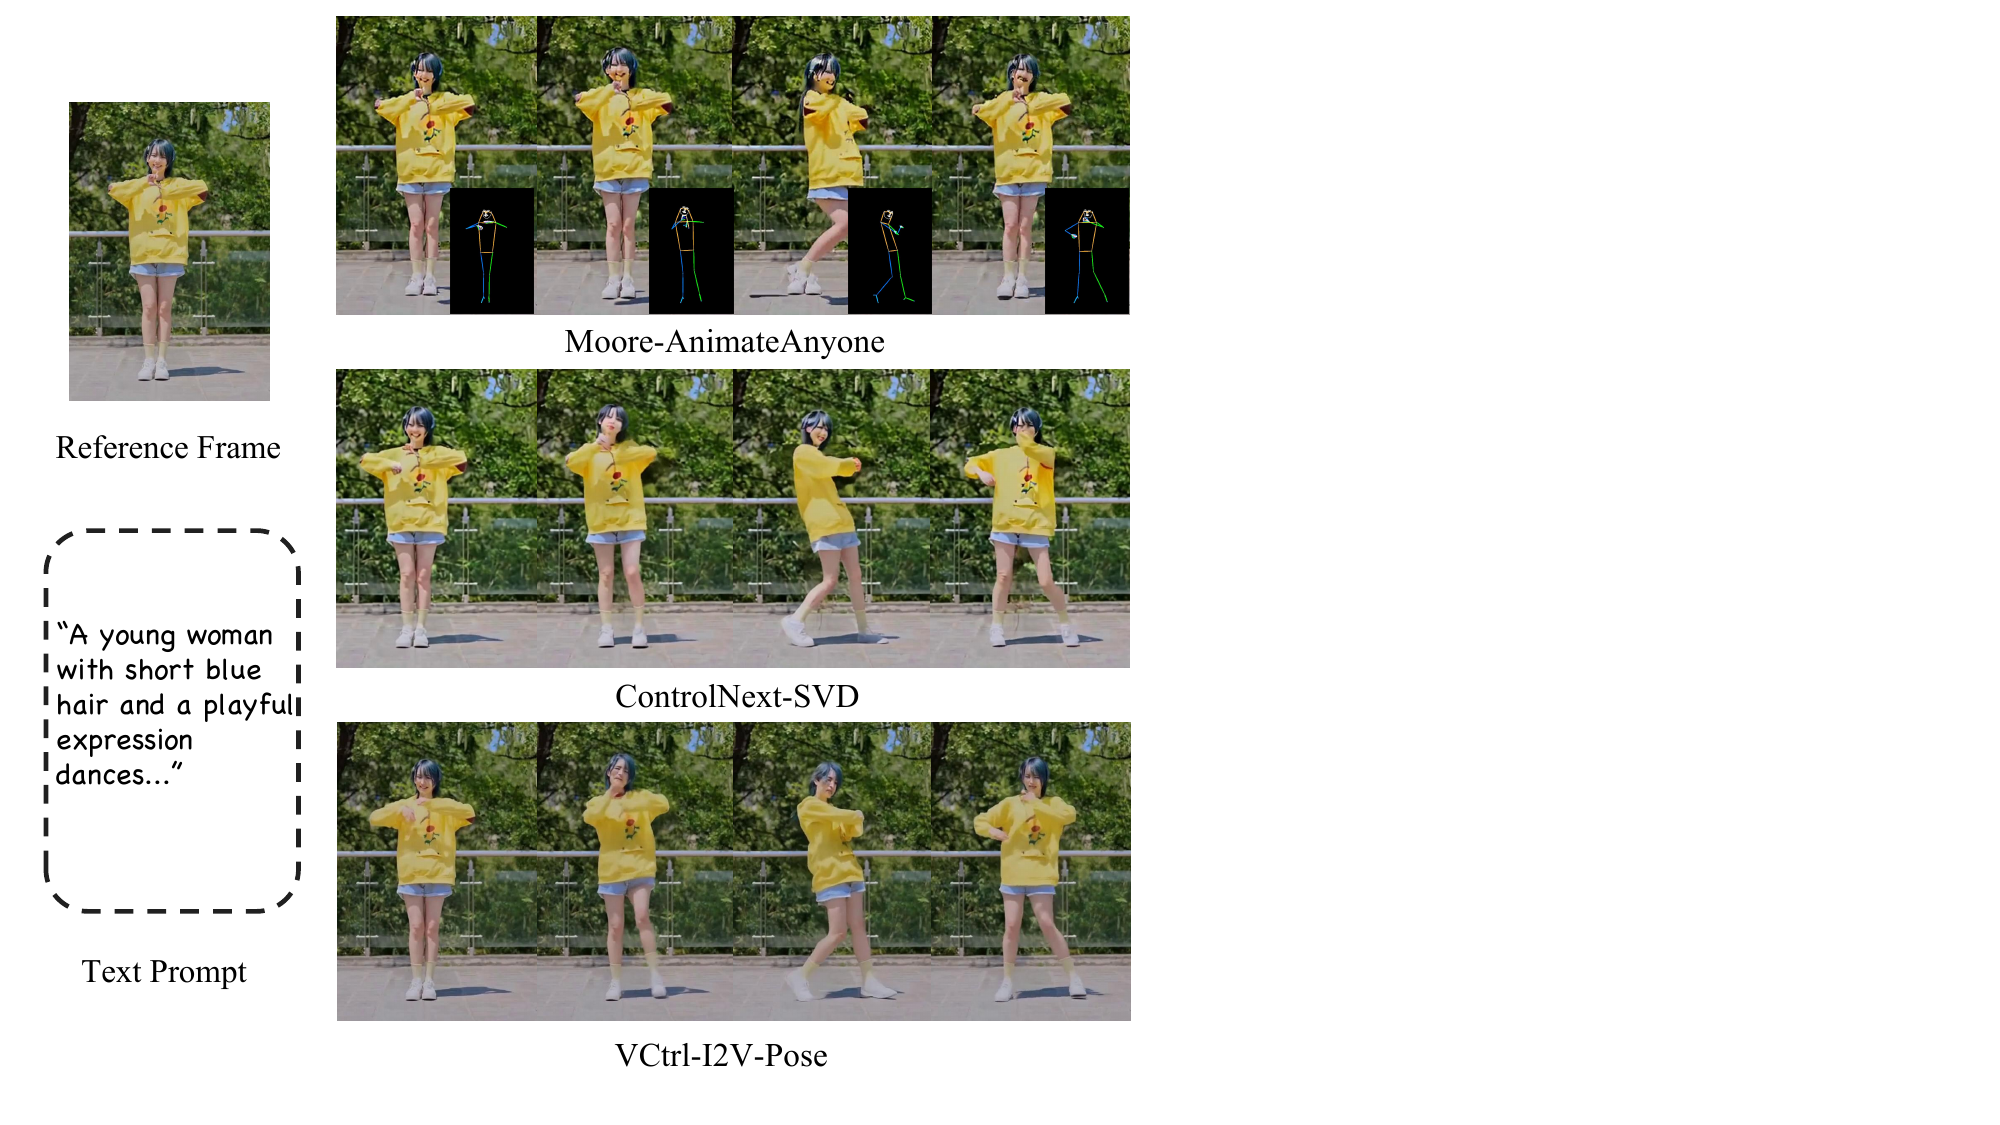}
    \vspace{-20pt}
    \caption{\textbf{Qualitative comparison to previous methods.} We compare our VCtrl-I2V-Pose with Moore-AnimateAnyone~\cite{moorethreads2024} and ControlNext-SVD~\cite{peng2024controlnext} on the Pose-to-Video task, showing that our model achieves superior visual quality and identity consistency.}
    \vspace{-7pt}
    \label{fig:pose_task}
\end{figure}

\begin{figure}
    \vspace{-3pt}
    \includegraphics[width=\linewidth]{./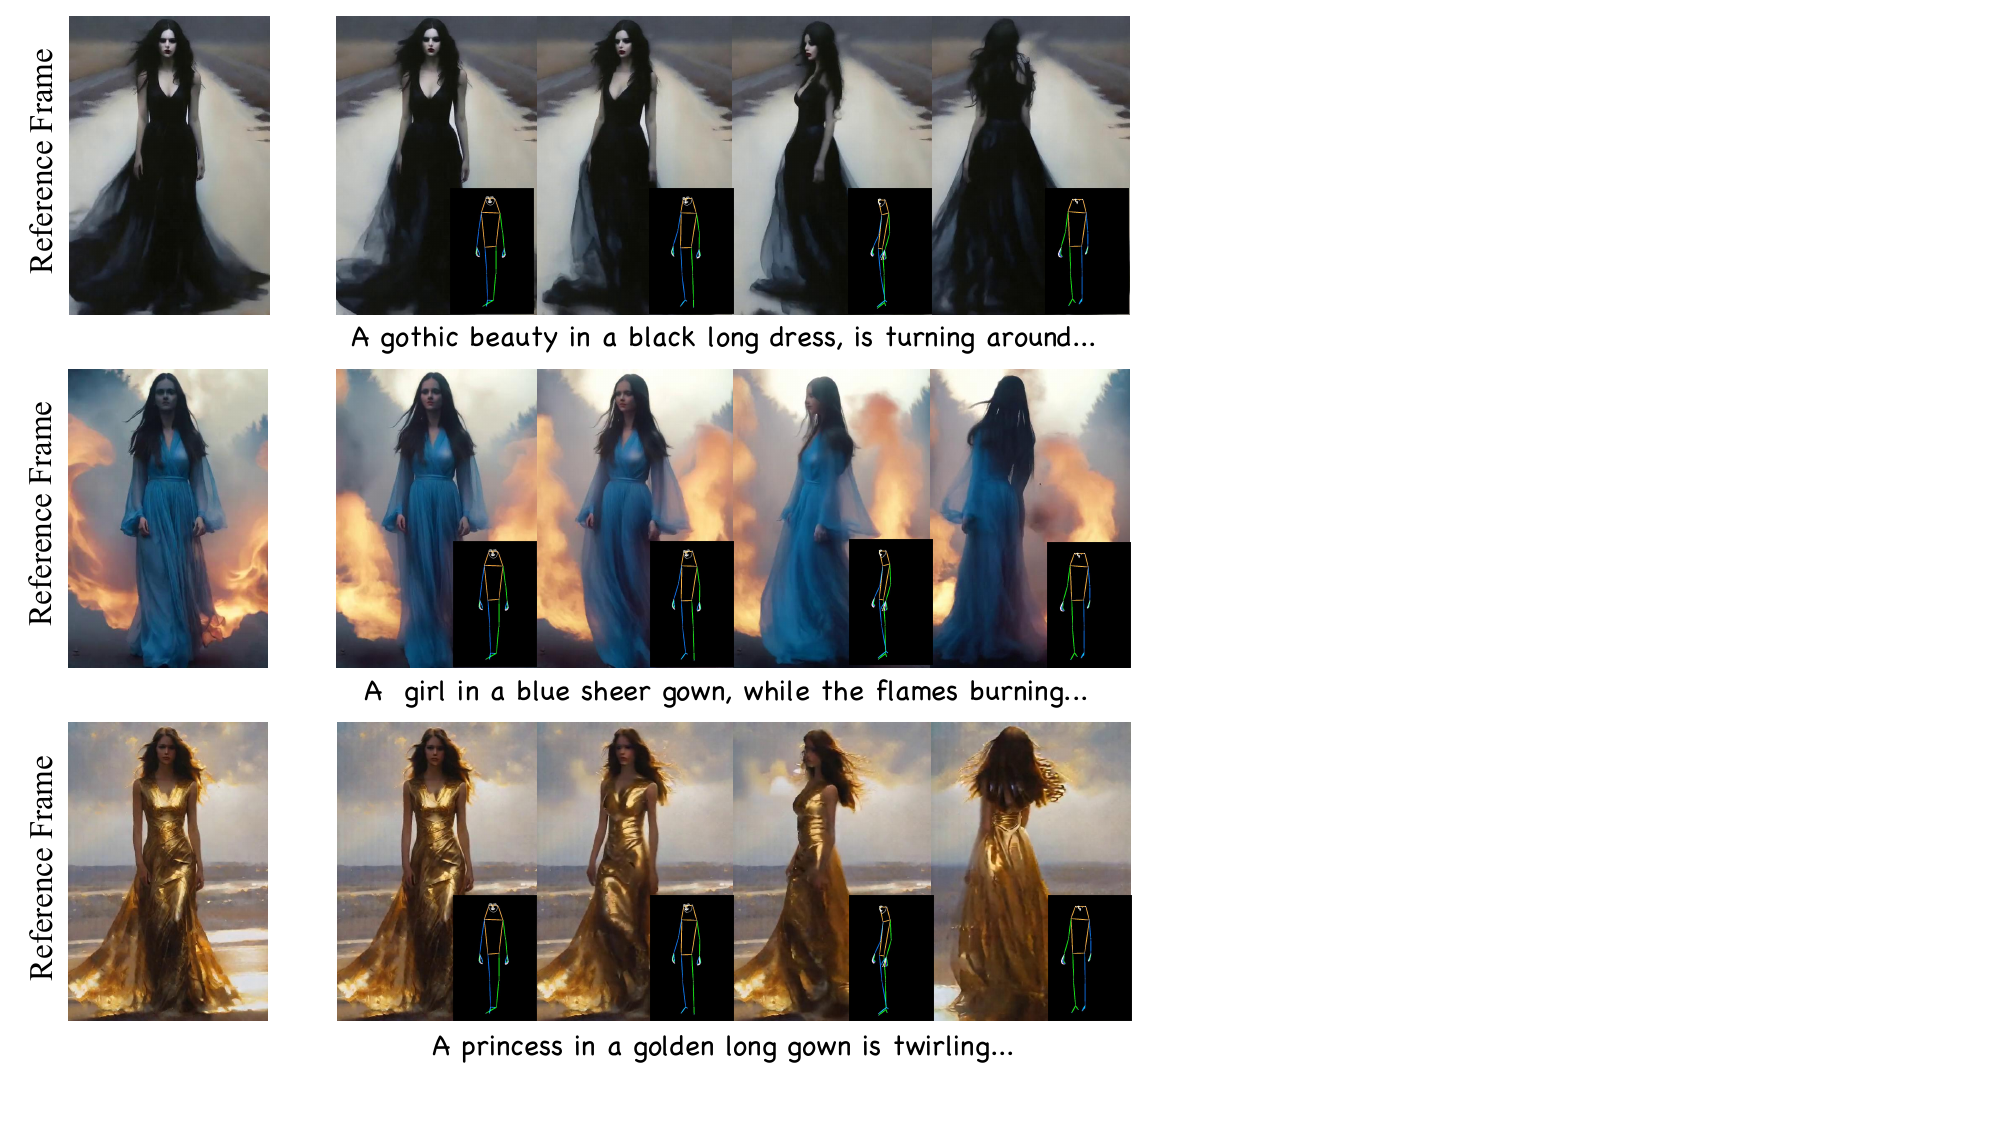}
    \vspace{-17pt}
    \caption{\textbf{Generalization Capability.} Conditioned on the same control signals, our model generates diverse, high-quality videos by varying the initial reference frame.}
    \vspace{-7pt}
    \label{fig:qualitive_results}
\end{figure}

In Figure~\ref{fig:mask_task}, we visually compare our models (VCtrl-Mask and VCtrl-I2V-Mask) against the representative baseline CoCoCo~\cite{zi2024cococo}. CoCoCo generates videos with noticeable inconsistencies in object appearance, resulting in visual artifacts and deviations from the textual description (e.g., incorrect vehicle color and texture). In contrast, our VCtrl-Mask precisely adheres to the semantic mask condition, significantly enhancing object consistency and visual realism. Furthermore, the I2V-enhanced variant (VCtrl-I2V-Mask) further improves visual fidelity, accurately matching the specified attributes (e.g., a brown jeep) and demonstrating superior temporal coherence across frames.

In Figure~\ref{fig:pose_task}, we present a qualitative comparison of our model (VCtrl-I2V-Pose) against representative baselines Moore-AnimateAnyone~\cite{moorethreads2024} and ControlNext-SVD~\cite{peng2024controlnext}.
Moore-AnimateAnyone exhibits noticeable temporal incoherence and poor adherence to the given pose, causing abrupt visual distortions. ControlNext-SVD maintains improved pose consistency but suffers from inconsistencies in appearance and noticeable artifacts. In contrast, our proposed VCtrl-I2V-Pose consistently achieves superior visual fidelity, precise alignment with the provided pose signals, and stable temporal coherence across frames, effectively preserving the initial identity throughout the sequence.

\subsection{Generalization} 
Our method demonstrates strong generalizability by generating diverse video outputs from the same control signals, achieved through altering the initial reference frame (Figure~\ref{fig:qualitive_results}). This capability underscores the flexibility and scalability of the proposed framework.
