# Supplementary material for: Enabling Versatile Controls for Video Diffusion Models
Source: arXiv:2503.16983 source file (2025-03-21)
Supplement: Supplementary file 2 [file main_suppl.pdf]

# VCtrl: Enabling Versatile Controls for Video Diffusion Models

## Supplementary Material

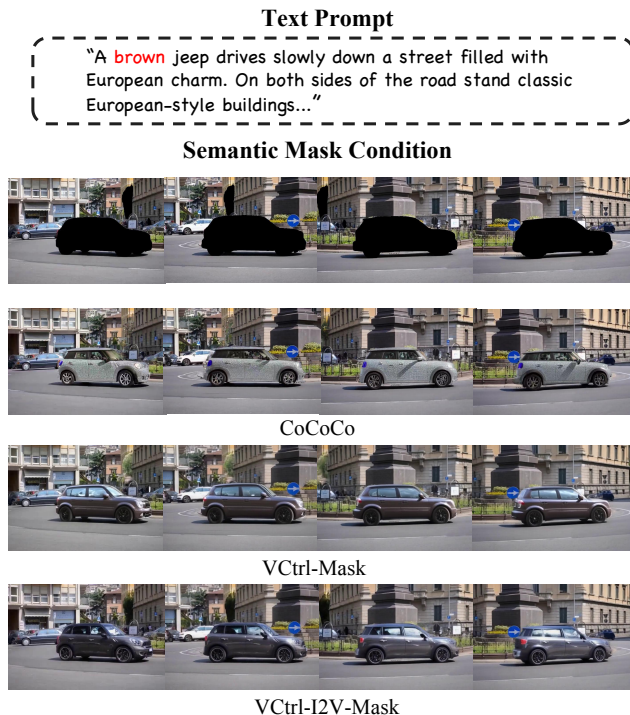

Figure 1. **Qualitative comparison to previous methods.** We compare our method with CoCoCo [3], demonstrating superior object consistency and stronger temporal coherence to the segmentation mask conditions.

## 1. Additional Results

### 1.1. Qualitative Comparison

In Figure 1, we visually compare our models (VCtrl-Mask and VCtrl-I2V-Mask) against the representative baseline CoCoCo [3]. CoCoCo generates videos with noticeable inconsistencies in object appearance, resulting in visual artifacts and deviations from the textual description (e.g., incorrect vehicle color and texture). In contrast, our VCtrl-Mask precisely adheres to the semantic mask condition, significantly enhancing object consistency and visual realism. Furthermore, the I2V-enhanced variant (VCtrl-I2V-Mask) further improves visual fidelity, accurately matching the specified attributes (e.g., a brown jeep) and demonstrating superior temporal coherence across frames.

In Figure 2, we present a qualitative comparison of our model (VCtrl-I2V-Pose) against representative baselines Moore-AnimateAnyone [1] and ControlNext-SVD [2]. Moore-AnimateAnyone exhibits noticeable temporal incoherence and poor adherence to the given pose, causing abrupt visual distortions. ControlNext-SVD maintains improved pose consistency but suffers from inconsistencies in appear-

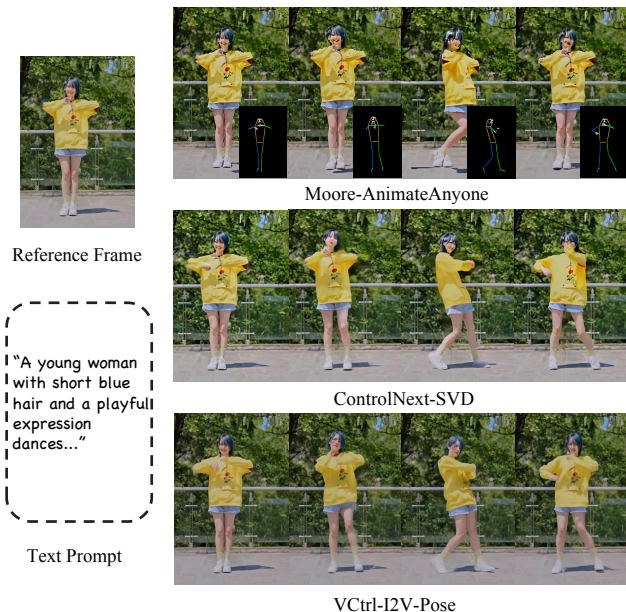

Figure 2. **Qualitative comparison to previous methods.** We compare our VCtrl-I2V-Pose with Moore-AnimateAnyone [1] and ControlNext-SVD [2] on the Pose-to-Video task, showing that our model achieves superior visual quality and identity consistency.

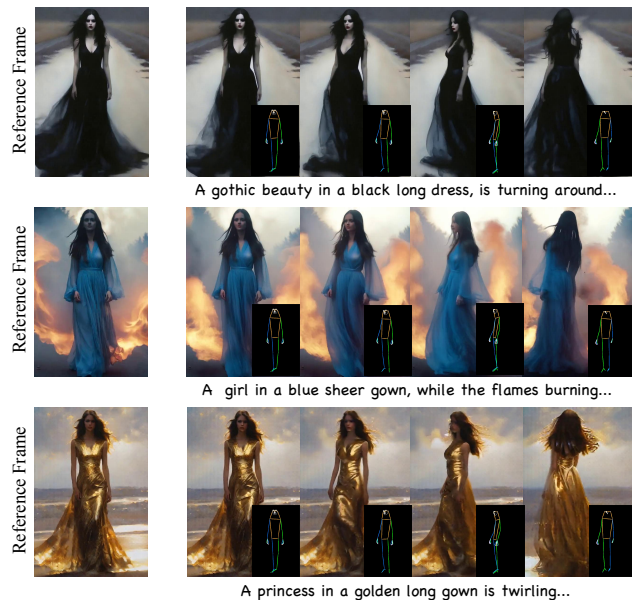

Figure 3. **Generalization Capability.** Conditioned on the same control signals, our model generates diverse, high-quality videos by varying the initial reference frame.

ance and noticeable artifacts. In contrast, our proposed VCtrl-I2V-Pose consistently achieves superior visual fidelity, precise alignment with the provided pose signals, and stable

temporal coherence across frames, effectively preserving the initial identity throughout the sequence.

## 1.2. Generalization

Our method demonstrates strong generalizability by generating diverse video outputs from the same control signals, achieved through altering the initial reference frame (Figure 3). This capability underscores the flexibility and scalability of the proposed framework.

## References

- [1] MooreThreads. Moore-animateanyone: Character animation (animateanyone, face reenactment). <https://github.com/MooreThreads/Moore-AnimateAnyone>, 2024. 1
- [2] Bohao Peng, Jian Wang, Yuechen Zhang, Wenbo Li, Ming-Chang Yang, and Jiaya Jia. Controlnext: Powerful and efficient control for image and video generation. *arXiv preprint arXiv:2408.06070*, 2024. 1
- [3] Bojia Zi, Shihao Zhao, Xianbiao Qi, Jianan Wang, Yukai Shi, Qianyu Chen, Bin Liang, Kam-Fai Wong, and Lei Zhang. Cococo: Improving text-guided video inpainting for better consistency, controllability and compatibility. *arXiv preprint arXiv:2403.12035*, 2024. 1
